# Supplementary material for: AttributionBench: How Hard is Automatic Attribution Evaluation?
Source: arXiv:2402.15089 source file (2024-02-23)
Supplement: Supplementary file 1 [file appendix_data_statistics.tex]

\begin{table}[t]
\resizebox{\linewidth}{!}{
\centering
\begin{tabular}{p{0.25\linewidth}<{\raggedright}p{0.2\linewidth}<{\raggedright}p{0.3\linewidth}<{\raggedright}p{0.3\linewidth}<{\raggedright}p{0.15\linewidth}<{\raggedright}p{0.15\linewidth}<{\raggedright}}

\toprule[1pt]
\multirow{2}{0.2\linewidth}{Version} & \multirow{2}{0.2\linewidth}{ExpertQA} & \multirow{2}{0.3\linewidth}{Stanford-GenSearch} & \multirow{2}{0.3\linewidth}{AttributedQA} & \multirow{2}{0.15\linewidth}{LFQA} & \multirow{2}{0.15\linewidth}{Total} \\
& & & & & \\
\cmidrule{1-6}
% \multirow{5}{0.25\linewidth}{Stanford-GenSearch} & \multirow{5}{0.76\linewidth}{AllSouls, davinci-debate, ELI5, WikiHow-Keywords, NaturalQuestions} & \multirow{5}{0.08\linewidth}{1510} & \multirow{5}{0.08\linewidth}{68} & \multirow{5}{0.08\linewidth}{148} \\ 
\multirow{2}{0.2\linewidth}{Subset-Balanced} & \multirow{2}{0.2\linewidth}{4442} & \multirow{2}{0.3\linewidth}{4784} & \multirow{2}{0.3\linewidth}{2000} & \multirow{2}{0.15\linewidth}{2096} & \multirow{2}{0.15\linewidth}{13.3k} \\
& & & & & \\
\cmidrule{1-6}
\multirow{2}{0.2\linewidth}{Overall-Balanced} & \multirow{2}{0.2\linewidth}{4764} & \multirow{2}{0.3\linewidth}{5196} & \multirow{2}{0.3\linewidth}{1665} & \multirow{2}{0.15\linewidth}{2087} & \multirow{2}{0.15\linewidth}{13.7k} \\
& & & & & \\
\cmidrule{1-6}
\multirow{2}{0.2\linewidth}{\makecell[Xl]{Not-Balanced}} & \multirow{2}{0.2\linewidth}{4945} & \multirow{2}{0.3\linewidth}{5440} & \multirow{2}{0.3\linewidth}{1452} & \multirow{2}{0.15\linewidth}{2163} & \multirow{2}{0.15\linewidth}{14.0k} \\
& & & & & \\
\cmidrule{1-6}
\multirow{3}{0.2\linewidth}{\makecell[Xl]{Not-Balanced\\(full data)}} & \multirow{3}{0.2\linewidth}{7671} & \multirow{3}{0.3\linewidth}{8673} & \multirow{3}{0.3\linewidth}{2208} & \multirow{3}{0.15\linewidth}{3319} & \multirow{3}{0.15\linewidth}{21.9k} \\
& & & & & \\
& & & & & \\
\bottomrule[1pt]
\end{tabular}
}
\caption{Data statistics of the label-balanced \texttt{AttributionBench}. ``Bal.'' denotes label-balanced or not. The label ratio (positive/negative) is 1:1 among all datasets. ``ID'' and ``OOD'' denotes "in-domain" and "out-of-domain", respectively.}
\label{tab:appendix_data_statistics}
\end{table}
