# Supplementary material for: AttributionBench: How Hard is Automatic Attribution Evaluation?
Source: arXiv:2402.15089 source file (2024-02-23)
Supplement: Supplementary file 2 [file appendix_id_results.tex]

\begin{table*}[ht]
\resizebox{\linewidth}{!}{
\centering
\begin{tabular}{ccl|cccc|c|ccc|c|c}

\toprule[1pt]
% \multirow{2}{0.2\linewidth}{\makecell[Xl]{Not-Balanced}}
% \multirow{2}{*}{Setting} & \multirow{2}{*}{\makecell{Training Set\\Version}} \\
 \multirow{2}{*}{\makecell{Model\\(size)}} & \multirow{2}{*}{Setting} & \multirow{2}{*}{\makecell{Training Set\\Version}} & \multirow{2}{*}{ExpertQA} & \multirow{2}{*}{\makecell{Stanford-\\GenSearch}} & \multirow{2}{*}{AttributedQA} & \multirow{2}{*}{LFQA} & \multirow{2}{*}{\makecell{ID-\\Avg.}} & \multirow{2}{*}{BEGIN} & \multirow{2}{*}{\makecell{AttrEval-\\GenSearch}} & \multirow{2}{*}{HAGRID} & \multirow{2}{*}{\makecell{OOD-\\Avg.}} & \multirow{2}{*}{\makecell{Overall-\\Avg.}} \\
 & & & & & & & & & & & & \\
 \cmidrule[1pt]{1-13}
& \text{C+E} & \makecell{\text{-}} & 55.3 & 62.0 & 74.7 & 72.6 & 66.2 & 79.4 & 76.7 & 70.1 & 75.4 & \textbf{70.1} \\
\multirow{3}{*}{GPT-3.5} & \text{Q+C+E} & \makecell{\text{-}} & 57.2 & 59.0 & 73.9 & 64.2 & 63.6 & 78.7 & 77.1 & 64.0 & 73.3 & 67.7 \\
& \text{C+E+R} & \makecell{\text{-}} & 42.8 & 44.9 & 58.1 & 39.3 & 46.3 & 72.4 & 40.9 & 58.2 & 57.2 & 50.9 \\
& \text{Q+C+E+R} & \makecell{\text{-}} & 48.6 & 48.1 & 70.2 & 53.1 & 55.0 & 74.2 & 70.5 & 56.1 & 66.9 & 60.1 \\
\cmidrule[1pt]{2-13}
& & \makecell{Subset-\\Balanced} & 60.5 & 80.2 & 79.9 & 85.6 & 76.6 & 84.1 & 83.3 & 73 & \textbf{80.1} & 78.1 \\
\cmidrule{3-13}
& \multirow{3}{*}{\text{C+E}} & \makecell{Overall-\\Balanced} & 61.7 & 82.3 & 82.1 & 83.5 & \textbf{78.3} & 85.5 & 85.2 & 67.7 & 79.5 & \textbf{78.8} \\
\cmidrule{3-13}
 & & \makecell{Not-Balanced} & 58.0 & 78.1 & 79.1 & 83.3 & 74.6 & 85.5 & 82.6 & 66.9 & 78.2 & 76.1 \\
\cmidrule{3-13}
 & & \makecell{Not-Balanced\\(full data)} & 55.6 & 78.3 & 79.1 & 83.9 & 74.2 & 81.8 & 82.6 & 63.2 & 75.9 & 74.9 \\
\cmidrule[1pt]{2-13}
 & & \makecell{Subset-\\Balanced} & 62.3 & 81.8 & 79.5 & 87.5 & \textbf{77.8} & 85.7 & 84.5 & 74.8 & \textbf{81.7} & \textbf{79.4} \\
\cmidrule{3-13}
  & \multirow{3}{*}{\text{Q+C+E}} & \makecell{Overall-\\Balanced} & 61.1 & 81.3 & 81.2 & 86.9 & 77.6 & 86.6 & 84.4 & 67.2 & 79.4 & 78.4 \\
\cmidrule{3-13}
 \multirow{7}{*}{\makecell{Llama-2\\(7B)}} & & \makecell{Not-Balanced} & 58.4 & 78.2 & 77.8 & 84.4 & 74.7 & 85.1 & 80.8 & 70.3 & 78.7 & 76.4 \\
\cmidrule{3-13}
 & & \makecell{Not-Balanced\\(full data)} & 55.5 & 76.9 & 81.3 & 83.3 & 74.3 & 81.8 & 73.8 & 59 & 71.5 & 73.1 \\
\cmidrule[1pt]{2-13}
 & & \makecell{Subset-\\Balanced} & 60.6 & 80.2 & 77.3 & 82.1 & 75.1 & 77.5 & 84.5 & 69.2 & \textbf{77.1} & \textbf{75.9} \\
 \cmidrule{3-13}
& \multirow{3}{*}{\text{C+E+R}} & \makecell{Overall-\\Balanced} & 58.9 & 82.3 & 79.9 & 83.3 & \textbf{76.1} & 86.4 & 80.7 & 58.9 & 75.3 & 75.8 \\
\cmidrule{3-13}
 & & \makecell{Not-Balanced} & 57.8 & 78.9 & 82.1 & 80.4 & 74.3 & 88.3 & 82.7 & 59.7 & 76.9 & 75.4 \\
\cmidrule{3-13}
 & & \makecell{Not-Balanced\\(full data)} & 54.5 & 77.9 & 78.9 & 81.3 & 72.7 & 83.5 & 81.5 & 65.4 & 76.8 & 74.5 \\
\cmidrule[1pt]{2-13}
 & & \makecell{Subset-\\Balanced} & 60.6 & 80.8 & 82.5 & 84.5 & \textbf{77.1} & 83.0 & 84.5 & 72.8 & 80.1 & \textbf{78.4} \\
\cmidrule{3-13}
 & \multirow{3}{*}{\text{Q+C+E+R}} & \makecell{Overall-\\Balanced} & 62.9 & 81 & 78 & 82.7 & 76.2 & 86.0 & 83.9 & 72.4 & \textbf{80.8} & 78.1 \\
\cmidrule{3-13}
 & & \makecell{Not-Balanced} & 55.3 & 79.1 & 77.8 & 78.4 & 72.7 & 85.3 & 84.6 & 58.8 & 76.2 & 74.2 \\
\cmidrule{3-13}
 & & \makecell{Not-Balanced\\(full data)} & 56.1 & 78.1 & 79.9 & 80.4 & 72.9 & 82.3 & 83.3 & 57.8 & 74.5 & 73.6 \\
\bottomrule[1pt]
\end{tabular}
}
\caption{We conducted ablation experiments to compare the influence of different input fields and training sets. Q, C, E, and R represent question, claim, evidence, and response, respectively. Label-balanced training sets can consistently outperform not-balanced ones, although consisting of fewer data. After fine-tuning, Q+C+E performs slightly better than C+E, indicating that fine-tuning might eliminate the ambiguity involved by adding questions to the input.
}
\label{tab:appendix-in-domain-results}
\end{table*}
