# Supplementary material for: AttributionBench: How Hard is Automatic Attribution Evaluation?
Source: arXiv:2402.15089 source file (2024-02-23)
Supplement: Supplementary file 3 [file appendix_gpt_results.tex]

\begin{table*}[ht]
\resizebox{\linewidth}{!}{
\centering
\begin{tabular}{ccl|cccc|c|ccc|c|c}

\toprule[1pt]
% \multirow{2}{0.2\linewidth}{\makecell[Xl]{Not-Balanced}}
% \multirow{2}{*}{Setting} & \multirow{2}{*}{\makecell{Training Set\\Version}} \\
 \multirow{2}{*}{\makecell{Model}} & \multirow{2}{*}{Setting} & \multirow{2}{*}{\makecell{Training Set\\Version}} & \multirow{2}{*}{ExpertQA} & \multirow{2}{*}{\makecell{Stanford-\\GenSearch}} & \multirow{2}{*}{AttributedQA} & \multirow{2}{*}{LFQA} & \multirow{2}{*}{\makecell{ID-\\Avg.}} & \multirow{2}{*}{BEGIN} & \multirow{2}{*}{\makecell{AttrEval-\\GenSearch}} & \multirow{2}{*}{HAGRID} & \multirow{2}{*}{\makecell{OOD-\\Avg.}} & \multirow{2}{*}{\makecell{Overall-\\Avg.}} \\
 & & & & & & & & & & & & \\
 \cmidrule[1pt]{1-13}
& & \makecell{Subset-\\Balanced} & 60.5 & 80.2 & 79.9 & 85.6 & 76.6 & 84.1 & 83.3 & 73 & \textbf{80.1} & 78.1 \\
\cmidrule{3-13}
\bottomrule[1pt]
\end{tabular}
}
\caption{We conducted ablation experiments to compare the influence of different input fields and training sets. Q, C, E, and R represent question, claim, evidence, and response, respectively. Label-balanced training sets can consistently outperform not-balanced ones, although consisting of fewer data. After fine-tuning, Q+C+E performs slightly better than C+E, indicating that fine-tuning might eliminate the ambiguity involved by adding questions to the input.
}
\label{tab:appendix-in-domain-results}
\end{table*}
