# Supplementary material for: AttributionBench: How Hard is Automatic Attribution Evaluation?
Source: arXiv:2402.15089 source file (2024-02-23)
Supplement: Supplementary file 4 [file appendix_ood_results.tex]

\begin{table*}[ht]
\resizebox{\linewidth}{!}{
\centering
\begin{tabular}{ccl|ccc|ccc|ccc|c}

\toprule[1pt]
\multirow{2}{*}{\textbf{Setting}} & \multirow{2}{*}{\textbf{Model (Size)}} & \multicolumn{3}{c|}{\textbf{BEGIN}} & \multicolumn{3}{c|}{\textbf{AttrEval-GenSearch}} & \multicolumn{3}{c|}{\textbf{HAGRID}} & \textbf{OOD-Avg.} \\ \cmidrule{3-12}
 & & F1 $\uparrow$ & FP $\downarrow$ & FN $\downarrow$ & F1 $\uparrow$ & FP $\downarrow$ & FN $\downarrow$ & F1 $\uparrow$ & FP $\downarrow$ & FN $\downarrow$ & F1 $\uparrow$ \\ \midrule[1pt]
\multirow{11}{*}{Zero-shot} & FLAN-T5 (770M) & 79.6 & 9.2 & 11.2 & 80.8 & 6.2 & 13.0 & 75.9 & 13.1 & 10.9 & 78.8 \\
 & FLAN-T5 (3B) & 80.2 & 13.3 & 6.4 & 82.0 & 6.2 & 11.7 & \textbf{79.0} & 16.9 & 3.8 & 80.4 \\
 & AttrScore-FLAN-T5 (3B) & 78.9 & 17.7 & 3.0 & 76.3 & 16.7 & 6.8 & 68.6 & 26.9 & 2.6 & 74.6 \\
 & FLAN-T5 (11B) & 72.3 & 25 & 1.1 & 78.1 & 16.7 & 4.9 & 64.5 & 30.6 & 2.0 & 71.6 \\
 & T5\_xxl\_true\_mixture (11B) & \textbf{86.4} & 4.8 & 8.7 & 76.4 & 2.5 & 20.4 & 78.6 & 14.4 & 6.8 & 80.5 \\
 & Flan-UL2 (20B) & 82.2 & 13.1 & 4.6 & \textbf{87.7} & 5.6 & 6.8 & 73.9 & 21.4 & 3.9 & \textbf{81.3} \\
\cmidrule{2-12}
 & AttrScore-Alpaca (7B) & 75.9 & 20.4 & 3.0 & 82.1 & 6.8 & 11.1 & 73.9 & 19.9 & 5.6 & 77.3 \\
 & GPT-3.5 (w/o CoT) & \textbf{79.4} & 15.8 & 4.4 & 76.7 & 18.5 & 4.3 & 70.1 & 25.2 & 2.8 & 75.4 \\
 & GPT-3.5 (w/ CoT) & 77.6 & 14.9 & 7.3 & 82.1 & 11.1 & 6.8 & 74.0 & 19.7 & 5.1 & 77.9 \\
 & GPT-4 (w/o CoT) & 77.5 & 19.7 & 2.1 & \textbf{84.3} & 14.2 & 1.2 & 72.1 & 23.9 & 2.8 & 78.0 \\
 & GPT-4 (w/ CoT) & 77.5 & 18.3 & 3.7 & 83.3 & 8.0 & 8.6 & \textbf{75.9} & 18.5 & 5.2 & \textbf{78.9} \\
\midrule[1pt]
\multirow{11}{*}{Fine-tuned} & Roberta-large-mnli (330M) & 60.9 & 6.2 & 27.2 & 65.1 & 26.1 & 11.8 & 61.3 & 9.2 & 28.4 & 62.4 \\
\cmidrule{2-12}
 & FLAN-T5 (770M) & 79.6 & 9.2 & 11.2 & 80.8 & 6.2 & 13.0 & 75.9 & 13.1 & 10.9 & 78.8 \\
 & FLAN-T5 (3B) & 80.2 & 13.3 & 6.4 & 82.0 & 6.2 & 11.7 & \textbf{79.0} & 16.9 & 3.8 & 80.4 \\
 & AttrScore-FLAN-T5 (3B) & 90.8 & 6.7 & 2.5 & \textbf{85.1} & 4.3 & 10.5 & 76.6 & 19.0 & 3.9 & \textbf{84.2} \\
 & FLAN-T5 (11B) & 90.6 & 7.8 & 1.6 & \textbf{85.1} & 4.3 & 10.5 & 67.7 & 27.1 & 3.4 & 81.1 \\
 & T5\_xxl\_true\_mixture (11B) & \textbf{91.5} & 7.1 & 1.4 & 81.4 & 6.2 & 12.3 & 77.3 & 18.6 & 3.6 & 83.4 \\
 & Flan-UL2 (20B) & 90.1 & 6.9 & 3.0 & \textbf{85.1} & 4.9 & 9.9 & 67.8 & 26.6 & 4.0 & 81.0 \\
\cmidrule{2-12}
 & Llama-2 (7B) & 84.1 & 10.6 & 5.3 & 83.3 & 6.8 & 9.9 & 73.0 & 22.5 & 3.5 & 80.1 \\
 & AttrScore-Alpaca (7B) & 85.1 & 9.2 & 5.7 & 81.9 & 4.3 & 13.6 & 76.4 & 18.3 & 4.9 & 81.1 \\
 & GPT-3.5 (w/o CoT) & \textbf{86.8} & 11.0 & 2.1 & 81.3 & 4.9 & 13.6 & \textbf{77.6} & 16.9 & 5.1 & \textbf{81.9} \\
\midrule
 & Avg. Gain $^{*}$ & 9.9 & -6.6 & -3.2 & 2.5 & -4.1 & 1.6 & 1.0 & 0.3 & -1.2 & 4.6 \\
\bottomrule[1pt]
\end{tabular}
}
\caption{The baseline performance (Macro-F1 score) with different models on the 3 out-of-domain tasks of
\texttt{AttributionBench-test}. The best performance within each setting is marked in \textbf{bold}. FP: false positive
percentage (the ground truth is ``not attributable'' but the model predicts ``attributable''). FN: false negative percentage (the ground truth is ``attributable'' but the model predicts ``not attributable''). OOD-Avg.: the average score of F1 on 3 ood tasks. ``$\uparrow$'' and ``$\downarrow$'' represent
higher and lower is better, respectively. $^*$: The ``Avg. Gain'' is calculated by averaging the performance gain of each
model after being fine-tuned compared to being zero-shot prompted. Fine-tuning on The results demonstrate the effectiveness of
fine-tuning on \texttt{AttributionBench-train} not only improves in-domain performance but also improves generalizability on unseen data.}
\label{tab:appendix-out-of-domain-results}
\end{table*}
